# Supplementary material for: Traffic Accident Risk Forecasting using Contextual Vision Transformers
Source: arXiv:2209.11180 source file (2022-09-20)
Supplement: Supplementary file 1 [file appendix.tex]

\clearpage

  \appendix 

This document is accompanying the submission \textit{\titlename}.
The information in this document complements the submission, and it is presented here for completeness reasons. It is not required for understanding the main paper, nor for reproducing the results.
 
\subsection{Model representation}
123
